# Supplementary material for: Gaussian deformations in graphene ribbons: flowers and confinement
Source: arXiv:1405.1962 source file (2014-07-04)
Supplement: Supplementary file 1 [file Suplementary.pdf]

# Supplemental Material: Electronic transport in graphene nanoribbons with a Gaussian deformation

R. Carrillo-Bastos,[1,2,3] D. Faria,[4] A. Latgé,[4] F. Mireles,[2] and N. Sandler[3]

[1]*Posgrado en Física de Materiales,*
*Centro de Investigación Científica y Educación Superior de Ensenada,*
*Apado. Postal 356, 22800 Ensenada, Baja California, México*

[2]*Centro de Nanociencias y Nanotecnología,*
*Universidad Nacional Autónoma de México,*
*Apdo. Postal 2681, 22800 Ensenada, Baja California, México*

[3]*Department of Physics and Astronomy and Nanoscale and Quantum Phenomena Institute,*
*Ohio University, Athens, Ohio 45701-2979, USA*

[4]*Instituto de Física, Universidade Federal Fluminense,*
*Niterói, Avenida Litorânea sn, 24210-340 RJ, Brasil*

## I. DEFORMATION POTENTIAL

In tight-binding models, strain deformations modify hopping parameters and onsite energies (due to changes in the crystal field). The change of onsite energies is modeled through a deformation (scalar) potential, a concept introduced by Bardeen and Shockley[1]. For carbon based materials, the deformation potential was first introduced by Suzuura and Ando[2] who, starting from the electron-phonon coupling, derived an expression valid in the long wavelength limit (acoustic phonons). Under these conditions, the deformation potential appears in the Hamiltonian as

$$V = g\left(\varepsilon_{xx} + \varepsilon_{yy}\right), \tag{1}$$

where $g$ is a coupling constant and $\varepsilon_{ii}$ stands for the strain tensor components in the $ii$ direction. This expression, like others also derived empirically[3], has been used in previous works to account for qualitative changes in band structures[4]. It is important to note that in all cases the reported values of the coupling constant $g$ range from 0 to $-20$ eV. This wide variation is attributed to the probable screening of the potential[5].

For the Gaussian deformation, considered in our study, the deformation potential obtained from Eq. 1 is:

$$V(r) = \frac{gA^2}{b^2}\left(\frac{2r^2}{b^2}\right)e^{\left(\frac{-2r^2}{b^2}\right)}. \tag{2}$$

In Fig. 1 we show the spatial dependence of the deformation potential given by Eq. 2, for a Gaussian deformation with amplitude $A = 1.4$ nm, width $b = 4.3$ nm, and constant coupling, $g = -3.0$ eV. This potential possesses axial symmetry and increases carrier confinement in an annular region. As a consequence, changes in local energies are expected in the conductance and DOS, but not in the features characterized by their angular dependence, such as the flower structure and the sub-lattice asymmetry reported in the manuscript. Because the value of the coupling constant $g$ is largely undetermined[5], it is instructive to analyze some limiting cases to obtain a range of variation for the quantities of interest. We present results from such studies below, obtained with several values of $g$ for conductance, DOS and LDOS for ribbons terminated with armchair and zigzag edges.

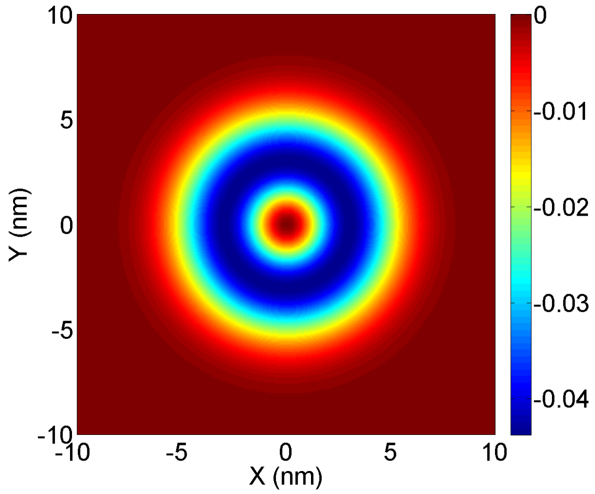


FIG. 1. (Color online) Deformation potential produced by a Gaussian bump with amplitude, $A = 1.4$ nm, width $b = 4.3$ nm and constant coupling, $g = -3.0$ eV.

### A. Conductance and DOS

The plots in Fig. 2 display results for conductance and DOS for five different situations for AGNR [panels a) and c)], and ZGNR [panels b) and d)]. For all the panels, the black dashed lines correspond to a ribbon without deformation and are plotted as reference. Blue curves correspond to a fully screened deformation potential ($g = 0$), while red, green and purple curves were produced including deformation potentials with coupling constants, $g = -1.0$ eV, $g = -2.0$ eV and $g = -3.0$ eV, respectively.

We first analyze the results for conductance, shown in panels a) and b). The main effect of the deformation is an overall decrease of the conductance with a degradation of the conductance steps as $|g|$ is increased. For larger values of $|g|$ two minima appear at energies close to inter-band transitions. The minima appearing exactly at energies of inter-band transitions (wider minima) become more pronounced with increasing values of $|g|$. This result supports the interpretation advanced in the paper that relates their origin to inter-band mixing enhanced by a perturbation (deformation potential). The narrower minima shift to lower energies with increasing values of $|g|$ (see the inset), consistent with the change in local energies mentioned above.

For each ribbon termination, conductance curves appear qualitatively similar for all the values of $g$ plotted. These results indicate that conductance profiles are independent of

specific value of $g$ and suggest that they are mostly determined by the pseudo magnetic field distribution (gauge field). Due to the differences between these distributions, ribbons with different edge terminations produce qualitative different conductance curves.

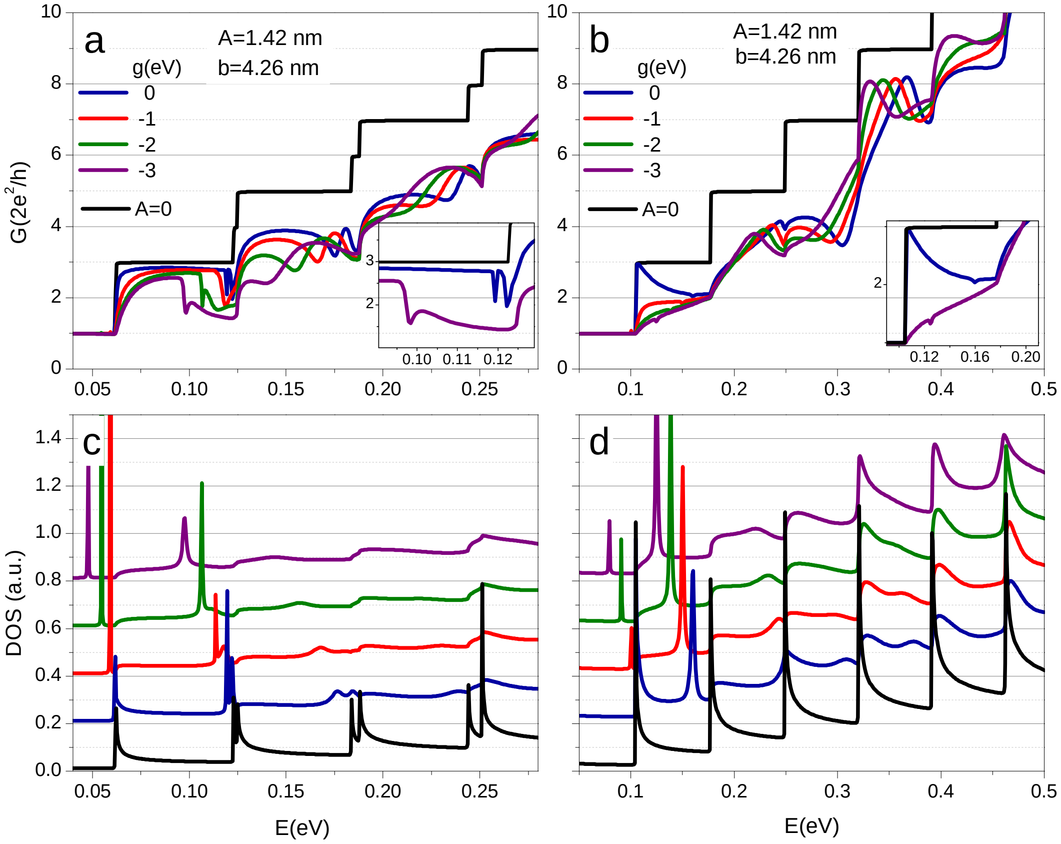


FIG. 2. (Color online) Effect of the deformation potential in the conductance and DOS for AGNR ($W$ = 30.0 nm, $L$ = 30.7 nm) [a) and b)], and ZGNR ($W$ = 25.8 nm, $L$ = 27.4 nm) [c) d)] nm for values of $g = -1.0$ (red), $-2.0$ (green), $-3.0$ (purple) eV. Gaussian deformation has amplitude $A$ = 1.4 nm and width $b$ = 4.3 nm. Black curves correspond to quantities without deformation. Blue curves are for $g = 0.0$ eV (corresponding to the blue curves appearing in Fig. 2 and Fig. 3 of the manuscript).

Changes in the DOS produced by the deformation potential with different values of $g$ can also be identified as shown in panels c) and d). As described in the main text, new confined levels arise as a spectral weight transfer from the original van Hove singularities occurs. As $|g|$ increases, these confined levels move towards lower energies tracking down the narrow minima in the conductance. This is a consequence of the local energy changes produced by

the deformation potential. Notice that for finite values of $g$ an additional peak at energies within the zero conductance plateau arises. Similar peaks are obtained for larger values of the amplitude $A$ (results not shown) without the deformation potential.

The above analysis leads to the conclusion that the effect of the deformation potential in the conductance and DOS can be generally described as an enhancement of the features produced by the pseudo-magnetic field described in the paper. As a final note we point out that in experimental settings, most probable values of $g$ would produce effects, in these two quantities, similar to those shown between the blue and the purple curves.

### B. LDOS and Local Pseudo-Spin Polarization

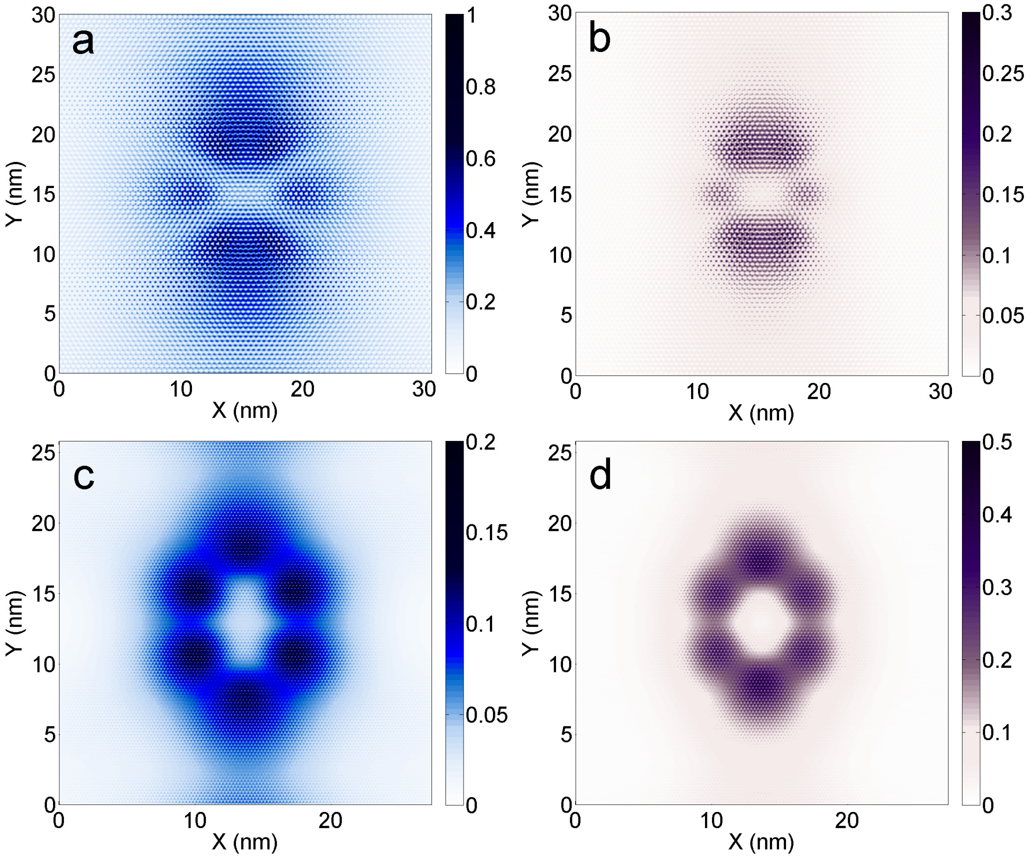


FIG. 3. LDOS with deformation potential for energies corresponding to minima in conductance (see inset in Fig.2). AGNR: a) $E = 0.119$ eV and $g = 0$, b) $E = 0.098$ eV and $g = -3$ eV. ZGNR: c) $E = 0.159$ eV and $g = 0$, d) $E = 0.124$ eV and $g = -3$ eV. Other system parameters are the same as those in Fig.2.

To understand the influence of the deformation potential on the LDOS we first study the changes in the LDOS at the energy values associated with the minima in the conductance. Fig. 3 shows data for LDOS for both edge terminations in the presence of a Gaussian deformation, without (left panels) and with (right panels) the deformation potential. As expected, the angular distribution of the enhanced LDOS region ('flower') is not modified by the deformation potential, but the structure has a smaller radial dimension. This indicates an increased confinement for larger deformation potentials as expected from Fig. 1.

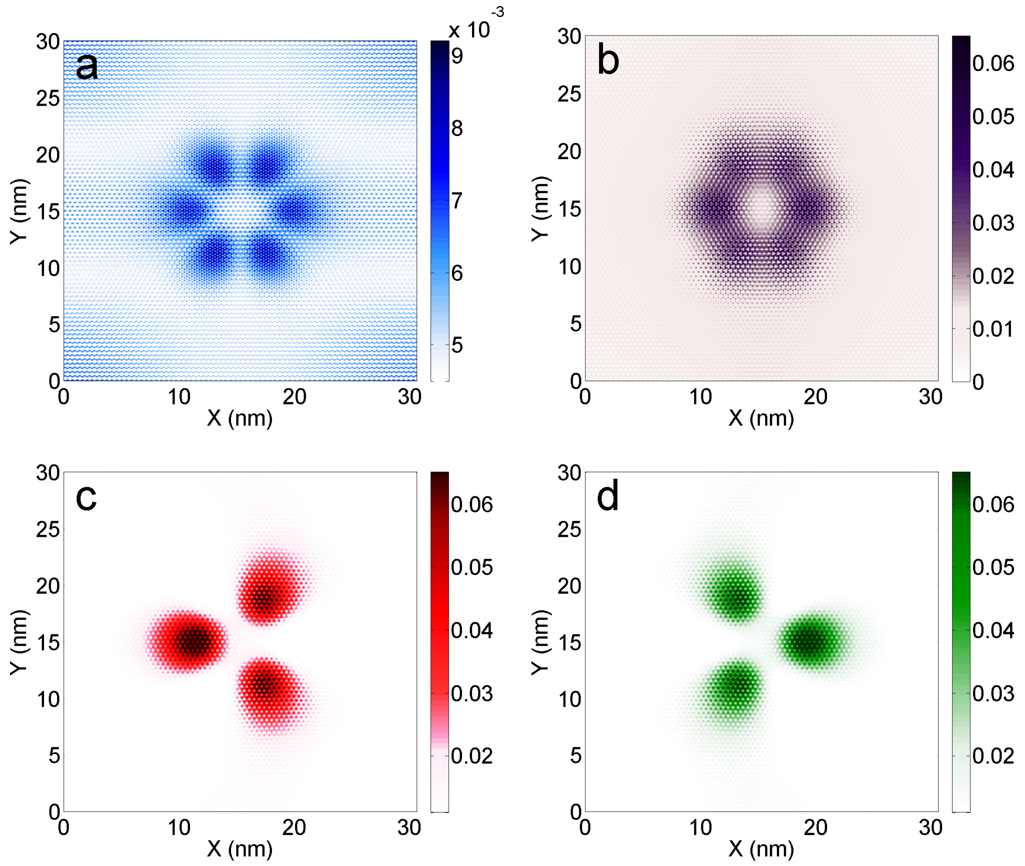


FIG. 4. Effect of the deformation potential on the LDOS for AGNR at fixed energy $E = 0.1$ eV with a) $g = 0$ and b) $g = -3.0$ eV. Panels c) and d) show data per sub-lattice, with $g = -3.0$ eV. Other system parameters are the same as those in Fig.2.

Finally, the deformation potential does not modify the existence of a pseudo-spin polarization (local sub-lattice symmetry breaking). This is exemplified by the data shown in Fig. 4 for an AGNR. Panel a) (Fig.4 in the paper) shows results for LDOS at energy $E = 0.1$ eV with $g = 0.0$ eV, while panel b) corresponds to the value $g = -3.0$ eV. It is clear from these figures that the only effect of the deformation potential is to shrink the whole struc-

ture in the radial direction. Moreover, panels c) and d) provide further evidence that the deformation potential preserves not only the six-fold symmetric pattern but also the local pseudo-spin polarization. Similar results are obtained for ZGNR (not shown).

In summary, the deformation potential introduces changes in the local energy scale, enhancing the confinement produced by the gauge field caused by the hopping modification. As a consequence its inclusion in the model Hamiltonian results in shifts of the energy positions of local minima and other features characterizing conductance and DOS. These shifts however, do not extend to features characterized by their angular dependence, such as the flower structure and the sub lattice asymmetry reported in the manuscript. These ones, having the same space symmetry as the gauge field, can only be produced by the change of hopping parameters introduced by strain. Therefore they will appear irrespective of the value of the coupling constant $g$.

---


[1] J. Bardeen and W. Shockley, Phys. Rev. **80**, 72 (1950).

[2] H. Suzuura and T. Ando, Phys. Rev. B **65**, 235412 (2002).

[3] J. V. Sloan, A. A. P. Sanjuan, Z. Wang, C. Horvath, and S. Barraza-Lopez, Phys. Rev. B **87**, 155436 (2013).

[4] G. M. M. Wakker, R. P. Tiwari, and M. Blaauboer, Phys. Rev. B **84**, 195427 (2011).

[5] M. Vozmediano, M. Katsnelson, and F. Guinea, Physics Reports **496**, 109 (2010).
